# Supplementary material for: Modelling spin-wave interference with electromagnetic leakage in micron-scaled spin-wave transducers
Source: arXiv:2509.24647 ancillary file (2025-09-29)
Supplement: Supplementary file 1 [file Supplemental_information_Crosstalk_impact_on_spin_wave_transducers.pdf]

# Supplementary information - Modelling spin-wave interference with electromagnetic leakage in micron-scaled spin-wave transducers

Felix Kohl,\* Björn Heinz, Matthias Wagner, and Philipp Pirro

*Fachbereich Physik and Landesforschungszentrum OPTIMAS,*

*Rheinland-Pfälzische Technische Universität Kaiserslautern-Landau, D-67663 Kaiserslautern, Germany*

Christoph Adelmann and Florin Ciubotaru

*imec, Kapeldreef 75, 3001 Heverlee, Belgium*

(Dated: September 29, 2025)

## I. FERROMAGNETIC RESONANCE

The calculations in the main text of the paper require knowledge of the effective saturation magnetization and the spin-wave damping of the YIG used. A broadband ferromagnetic resonance measurement was carried out on the sample to determine this. An exemplary transmission spectrum for an external field of  $H_{\text{ext}} = 144.7 \text{ mT}$  is shown in the inset of Figure S1 a) after subtracting a reference measurement. To extract the resonance frequency and the linewidth of the resonance, the real and imaginary parts are fitted using the equation from [1]. The resonance frequency obtained as a function of the external field is shown in S1 a). Fitting the Kittel equation [2]

$$f = \gamma \mu_0 \sqrt{H_{\text{ext}}(H_{\text{ext}} + M_{\text{s}}^{\text{eff}})} \quad (\text{S1})$$

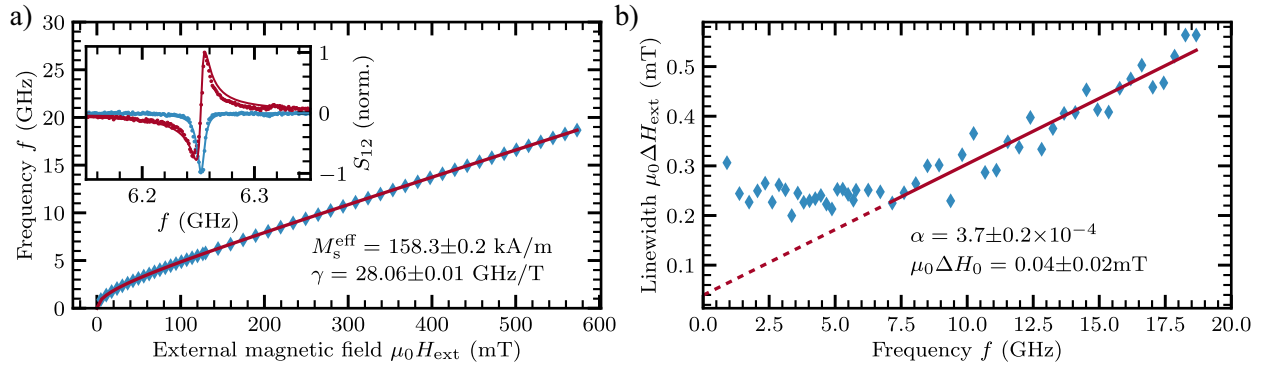

FIG. S1. a) Ferromagnetic resonance frequency as function of the externally applied magnetic field. The parameters obtained from fitting the Kittel equation to the data are indicated in the figure. The inset shows the real (blue) and imaginary part (red) of the  $S_{12}$  parameter along with the fitted function used to extract resonance frequency and linewidth. b) Calculated field-linewidth from the broadband ferromagnetic resonance measurement, along with a linear fit to the data to obtain Gilbert damping parameter and inhomogeneous linewidth indicated in the plot. Data points below 7 GHz are excluded from the fit, indicated by a dotted line.

provides the values of the gyromagnetic ratio  $\gamma$  and the effective saturation magnetization  $M_{\text{s}}^{\text{eff}}$ , used for the calculations in the further course of the work. The linewidths  $\Delta f$  of the measured resonances can be converted into effective field line widths  $\Delta H$  using the relation [1]:

$$\Delta H = \Delta f \frac{\partial H_{\text{res}}(f)}{\partial f} \Big|_{f=f_{\text{res}}} \quad (\text{S2})$$

For these, a linear dependence on the resonance frequency can be assumed [1] and a linear approximation

\* [fkohl@rptu.de](mailto:fkohl@rptu.de)

$$\Delta H = \Delta H_0 + \frac{4\pi\alpha f}{|\gamma|} \quad (\text{S3})$$

yields the values for the Gilbert damping parameter  $\alpha$  and the inhomogeneous linewidth  $\Delta H_0$ .

## II. SPIN-WAVE EXCITATION EFFICIENCIES

In the main text of the paper, three different antenna types are investigated. As outlined in [3], the shape of the measured spin-wave transmission spectrum is predominantly determined by the wave-vector distribution of the antenna fields used for the excitation and detection. The field distribution for each of the antennas used in the experiment is calculated assuming rectangular wires with homogeneous current distribution using the Biot-Savart law. Then a Fourier transform is applied to the field profile in real space to obtain the wave-vector distribution. The respective excitation efficiencies, obtained using the antenna dimensions given in Table S1, are shown in the top row of Fig. S2 alongside with the calculated dispersion relation in Damon-Eshbach configuration for an external field of 143 mT. From the figure, it can be seen that each of the antennas used has their respective maximum around the same wave-vector. While the GS and GSG wave-vector distributions look similar with one main maximum and fastly decreasing higher order maxima, for the GSGS antenna the spectrum is more complex, showing an amplitude modulation of the higher order maxima. This can be explained by the modulation of the GS spectrum due to the folding into the meander shape.

For a better comparison to the experiment, the bottom row of Fig. S2 shows the calculated transmission spectra

TABLE S1. Dimensions for the antennas investigated in the experiment. The meander antenna is obtained by folding the GS antenna once and keeping the same distances between all metal lines.

| Antenna | Ground $w_g$ ( $\mu\text{m}$ ) | Signal $w_s$ ( $\mu\text{m}$ ) | Spacing $s$ ( $\mu\text{m}$ ) |
|---------|--------------------------------|--------------------------------|-------------------------------|
| GS      | 2                              | 2                              | 4                             |
| GSG     | 2.5                            | 2.5                            | 2                             |
| Meander | 2                              | 2                              | 4                             |

for the unperturbed case and propagation distance  $D = 50 \mu\text{m}$ , assuming only neglectably small electromagnetic crosstalk (EM) levels, at an external magnetic field of 143 mT. The transmission spectrum in dB is calculated from the calculated  $Z$ -matrix according to the well known conversion [4]

$$S_{21}(\text{dB}) = 20 \cdot \log_{10} \left( \left| \frac{2Z_0 Z_{21}}{(Z_{22} + Z_0)(Z_{11} + Z_0) - Z_{12} \cdot Z_{21}} \right| \right). \quad (\text{S4})$$

using  $Z_0 = 50 \Omega$  as the port reference impedance,  $Z_{11} = Z_{22} = i\omega L_m$  and  $Z_{ij} = i\omega \mathcal{M}$  only considering the respective sign of  $k$  for the integral. The shape of the spectra resembles the shape of the wave-vector spectra, but is distorted due to the mapping of the wave-vector distribution to the frequency regime via the spin-wave dispersion relation. Both, the GS and the GSG antennas exhibit a pronounced main maximum of spin-wave transmission, corresponding to low-wave-vector peak in the antenna wave-vector distribution. Contribution of higher order excitation peaks to the transmission is reduced due to the vanishing group velocity at larger wave vectors. For the meander antenna, apart from the main peak, at low wave-vectors there are several small side peaks, that lead to a more complex shape of the transmission spectrum, as all these peaks are in the regime of high group velocity in the dispersion relation. Consequently they are less affected by damping losses during propagation as the side peaks for the GS and GSG antenna. Therefore they can contribute to the spin-wave transmission.

## III. ANALYTIC CALCULATION OF INDUCED PASSBAND RIPPLE

In the main text, the modulation of the transmitted signal observed in the experiment is attributed to the interference of EM with the spin waves. Thus, the modulation directly depends on the relative magnitude of the two contributions as well as the propagation distance and the spin-wave dispersion. These are considered in more detail in this section.

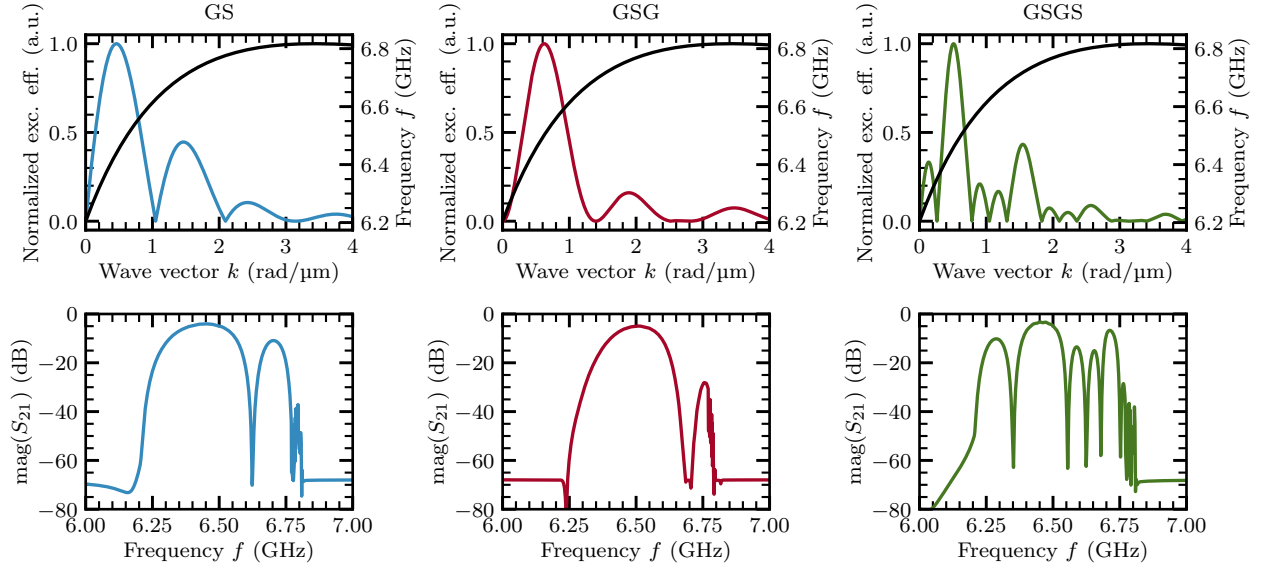

FIG. S2. Top row: Wave-vector dependent excitation efficiencies defined by the Fourier transform of the antenna field for all three antenna types investigated in the main text. Shown in black is the dispersion relation calculated for an external field of 143 mT, saturation magnetization  $M_s = 158.3$  kA/m and an exchange constant  $A_{\text{ex}} = 3.5$  pJ/m<sup>3</sup>. Bottom row: Resulting calculated transmission spectra, assuming a constant electromagnetic crosstalk impedance of  $0.01 \Omega$ .

### A. Scaling crosstalk magnitude

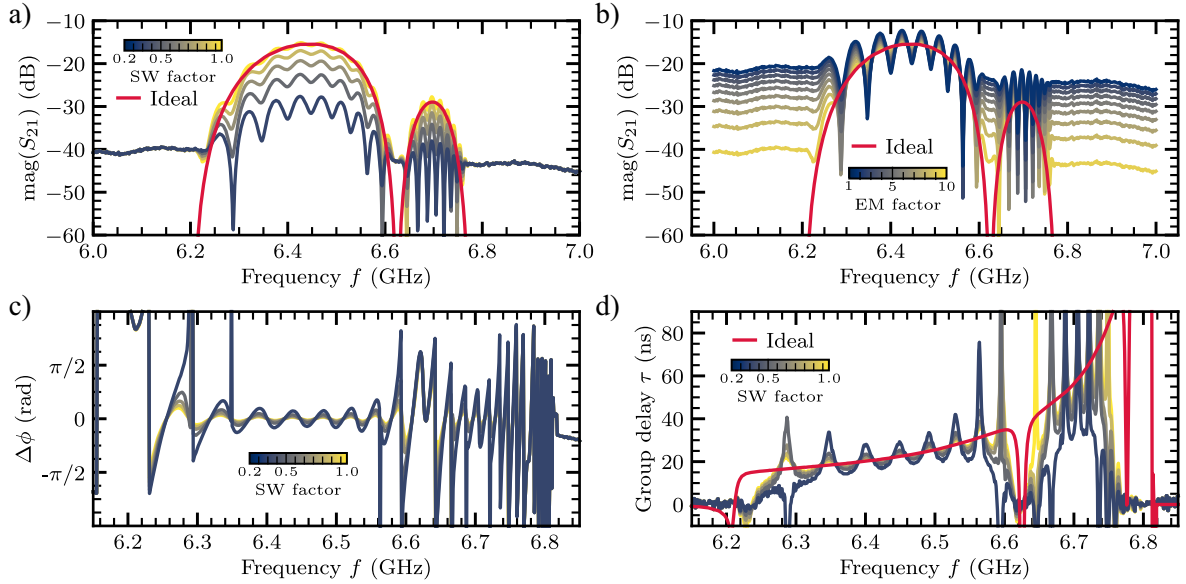

FIG. S3. Calculated transmission spectra for GS antenna on 500 nm thick YIG film with  $M_s = 158.3$  kA/m and  $A_{\text{ex}} = 3.5$  pJ/m<sup>3</sup> in an external field of 143 mT for a) scaled spin-wave impedance and b) scaled EM. Shown in red is the ideal case of zero crosstalk. c) Calculated difference in phase to the ideal case and corresponding group delay (d)) for scaled spin-wave impedance and the ideal case in red.

First, the influence of a scaled magnitude ratio between the spin wave contributions and the EM contribution is considered. Figure S3 shows the effects of varying the spin-wave impedance (a), c) and d)) and the EM (b)). The unperturbed case is marked in red in each figure. For Fig. S3 a), as the mutual spin-wave impedance is decreased, the total transmission magnitude decreases and the modulation of the magnitude increases. In contrast, an increase in the crosstalk leads to a stronger background signal as seen in Fig. S3 b), which increasingly masks the spin-wave signal.

The decisive factor for the resulting modulation is not the absolute strength, but the ratio of spin-wave impedance to crosstalk contribution. However, adjusting the ratio not only affects the modulation in magnitude, but also increases the influence on the phase modulation (see Fig. S3 c) using the scaled spin-wave contribution) and the resulting distortion in the group delay (see Fig. S3 d)), which has already been discussed in the main text. A scaled spin-wave impedance leads to an increasing modulation for both of these quantities, which can exceed the magnitude of the undisturbed value, especially in the case of the group delay.

### B. Impact of spin-wave propagation distance

While the EM undergoes almost no frequency-dependent phase accumulation over the typical propagation distances, the spin waves accumulate a strongly frequency-dependent phase due to their significantly varying wave-lengths on the order of a few microns. This phase is described by  $\phi = k \cdot D$ , with the propagation distance  $D$ . Points of constructive (destructive) interference occur at a relative phase accumulation difference of  $2\pi = k \cdot D$ . While the distance between these points is constant in wave-vector space, in the experiment the periodicity is mapped into frequency space using the non-linear spin-wave dispersion relation. The relation also directly shows that the periodicity depends on the propagation distance.

As an illustration for the dependence on the propagation distance  $D$ , Fig. S4 a) shows the transmission spectra calculated with the model from the main text for different propagation distances between  $50\text{ }\mu\text{m}$  and  $200\text{ }\mu\text{m}$ . Qualitatively, the spectra are similar in all cases. The increasing attenuation of the spin waves with increasing distance significantly reduces the amplitude of the second maximum, in particular. At the same time, the frequency of the modulation increases noticeably with increasing distance, leading to blurring of the secondary maximum at the greater distances. To analyze the periodicities quantitatively, they were extracted from the transmission spectra and shown in Fig. S4 b). The general trend of shorter periods at higher frequencies is due to the decreasing group velocity of the spin waves in the Damon-Eshbach dispersion. A constant  $\Delta k$ , corresponding to a phase difference of  $2\pi$ , spans over a smaller frequency interval at the low group velocity. Therefore, constructive or destructive interference points in the spectrum occur closer together at higher frequencies than at lower frequencies. As the propagation distance  $D$  increases, the distance between these interference points decreases continuously over the entire frequency band, due to the faster phase accumulation. The solid lines in Fig. S4 b) are calculated using only the dispersion relation by extracting the difference in frequency for points of relative differences in phase accumulation of  $2\pi$ .

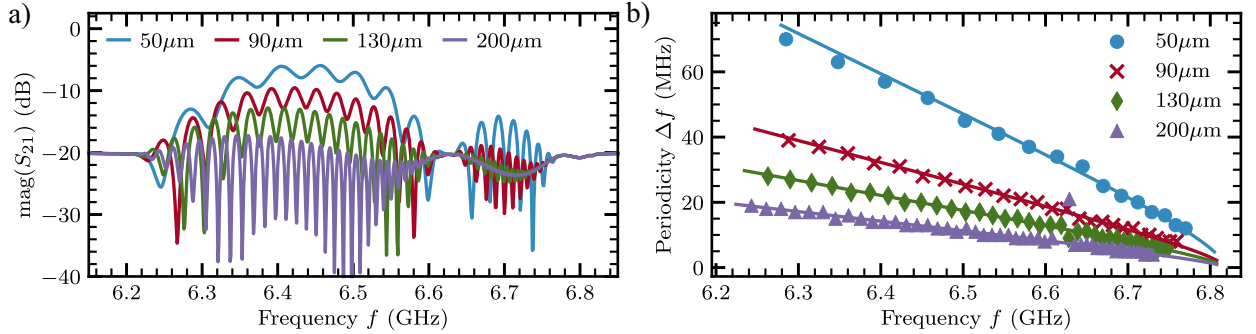

FIG. S4. a) Calculated spin-wave transmission spectra for different propagation distances  $D$  using the same parameters and field as above and assuming a constant electromagnetic crosstalk impedance of  $2\Omega$  and  $\alpha = 2.5 \cdot 10^{-4}$ . The periodicities of the resulting modulation for all distances are shown in b). Solid lines mark the expected periodicities extracted from the dispersion relation for frequency pairs with a relative phase shift of  $\Delta k \cdot D = 2\pi$

### C. Field dependence for constant crosstalk

Using the analytic model, the impact of changing the external field can also be evaluated. For simplicity, the EM dependency is set constant. The resulting spin-wave transmission spectra for different external magnetic fields are shown in Fig. S7 a). Two features can be observed. The first one is, that although the level of EM is set to be constant and transmission amplitude does not increase significantly, the resulting modulation in the spin-wave transmission is decreasing for higher frequencies. This can be explained by referring to the inductive nature of the model used to calculate the spin-wave impedances taken from [5]. Consequently, for increasing frequency as long as the decay length

is large, the spin-wave contributions to  $Z_{21}$  and  $Z_{12}$  increase with frequency. Therefore, the relative magnitude of the EM compared to the spin-wave impedances is decreased for higher frequencies, leading to weaker modulation. The second observation directly relates to the periodicity of the modulation. An increase in the external magnetic field results in a flattening of the spin-wave dispersion relation, as shown by the reduced group velocities in Fig. S7 b). Although the spin-wave phase accumulation during the propagation remains the same for all the fields considered, the flatter dispersion maps the constant modulation in wave-vector space to an decreasing interval in frequency space, resulting in faster modulation. This is shown in Fig. S7 c). A significant reduction can be observed.

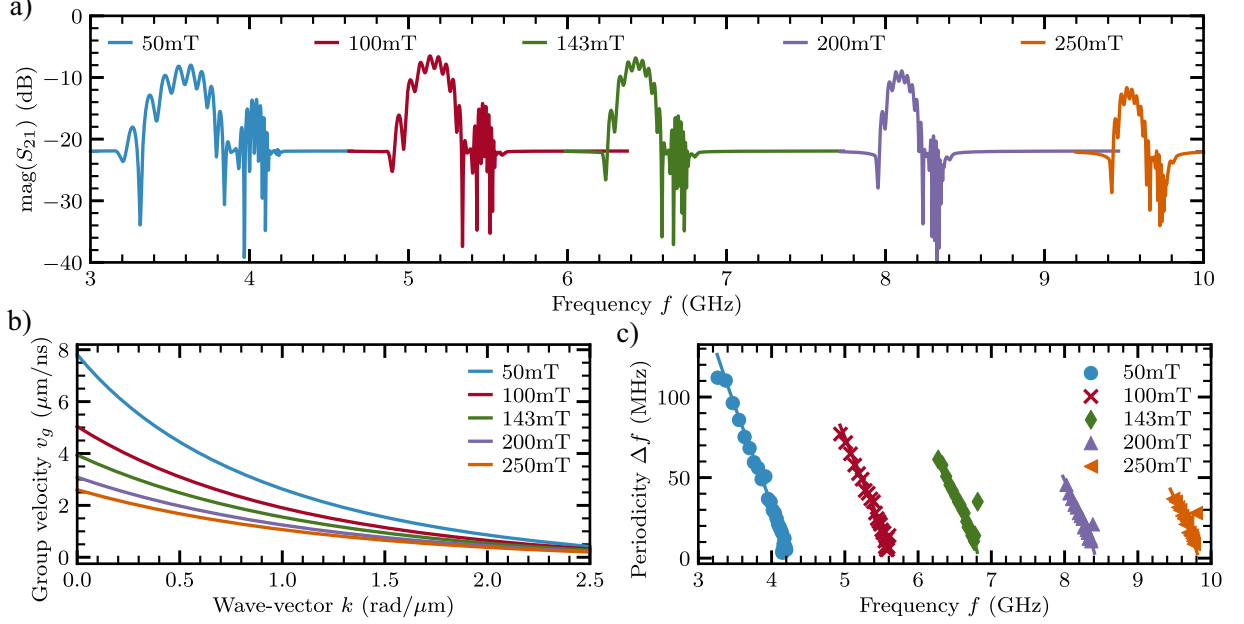

FIG. S5. a) Calculated spin-wave transmission spectra for different external magnetic fields and fixed edge-to-edge distance  $D = 50 \mu\text{m}$ . b) Group velocities calculated for the same fields as in a). The extracted periodicities in the modulation from a) are shown in c). Due to decreasing group velocity, periodicities are decreasing for increasing external magnetic field.

#### IV. MEASURED NONRECIPROCITY

In the main text, it has already been shown for the direction of strong transmission in the experiment that the influence of the EM can be eliminated using the time gating described in [6] and consequently the modulation due to the interference is removed. In the experiment, however, the other, weaker spin-wave transmission direction  $S_{12}$  is also measured. The analytical calculation using the presented model already shows a qualitative difference for this case, as the spin-wave impedances are significantly lower than for the  $S_{21}$  direction. Thus, the contribution of the interference is not expressed by a (weak) modulation of the spin-wave signal, but by a strong modulation of the EM signal. The measured time response and the measured transmission spectrum together with the filtered spectrum after removing the first 5 ns are shown in Fig. S6 a) and b) for the case of the GS antenna and an external field of 143 mT. The time response is qualitatively identical to the case of strong transmission in the main text, but with much weaker spin-wave signals. The measured modulated spectrum coincides with the analytical calculation from the main text. The influence of the EM can eventually be filtered by timegating the data and the pure spin-wave transmission spectrum, similar to the case of strong transmission, is obtained. The same behavior is also observed for the group delay  $\tau$  in Fig. S6 c). In the unfiltered data, the quasi-constant contribution of the EM to the group delay dominates and the spin wave contribution only leads to an oscillation of the group delay around zero. After removing the EM, however, the previously measured course of the group delay is qualitatively restored.

#### V. MEASURED PHASE DISTORTION

In the main text, the EM interference impact on the transmission magnitude is presented analytically and experimentally. For the analytic calculation of the transmission spectrum, significant phase accumulation is observed within

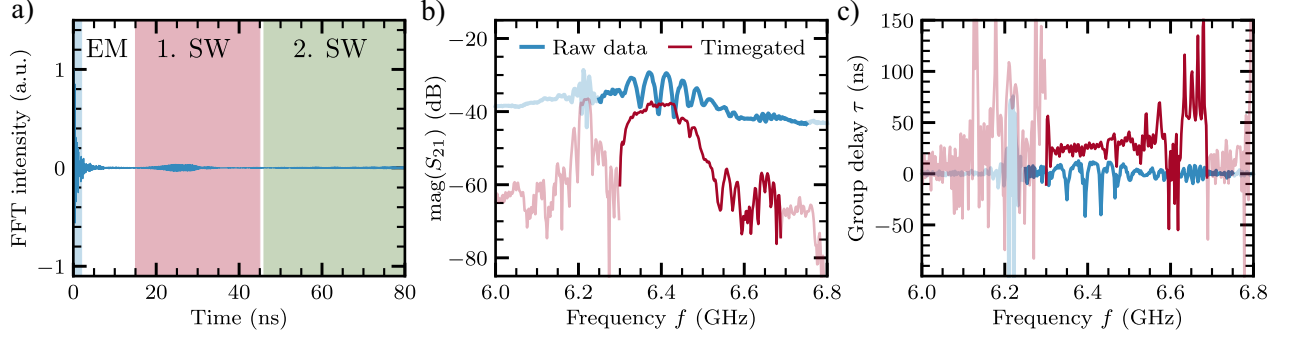

FIG. S6. a) Timetrace calculated from the frequency spectrum measured in b) for the GS antenna at an external field of 143 mT in the backward transmission direction  $S_{12}$ . The arrival times of the electric crosstalk and the spin-wave packets corresponding to the first and second antenna maximum are shaded in color. b) Measured transmission spectrum along with the spectrum obtained by setting the electric crosstalk to zero in a) and transformation back to the frequency domain. The spin-wave signal can be partially recovered by this. The off-band frequencies are shaded. c) Group delay directly calculated from the measured data along with the calculation using the timegated data. The initial slope of group delay caused by the spin-waves can be recovered from the timegated data.

the spin-wave transmission band for the case of strong spin-wave transmission. The effect of the EM interference in the phase is only weak and can only be seen in the difference phases of the perturbed and unperturbed cases. The same behaviour is also observed experimentally for the same experimental parameters as used for the calculation. The obtained data is shown in Fig. S5 a). The insets in the plot show zoomed in parts of the accumulated phase. Again, due to the large spin-wave amplitude and the weak EM, the modulation is weak. However, due to the nonreciprocal excitation and detection of spin-waves in the Damon-Eshbach configuration, the case of weak spin-wave amplitudes and weak EM can also be tested within the same measurement by inverting the spin-wave propagation direction, corresponding to the  $S_{12}$  trace. The corresponding accumulated phase is shown in Fig. S5 b). Here, due to the dominating EM contribution, no phase accumulation similar to the  $S_{21}$  trace is observed. Instead the phase varies only slightly across the spectrum and exhibits pronounced modulations inside the spin-wave transmission band. This observation underlines, the importance of the ratio between spin-wave and EM contributions for the effect of the modulation.

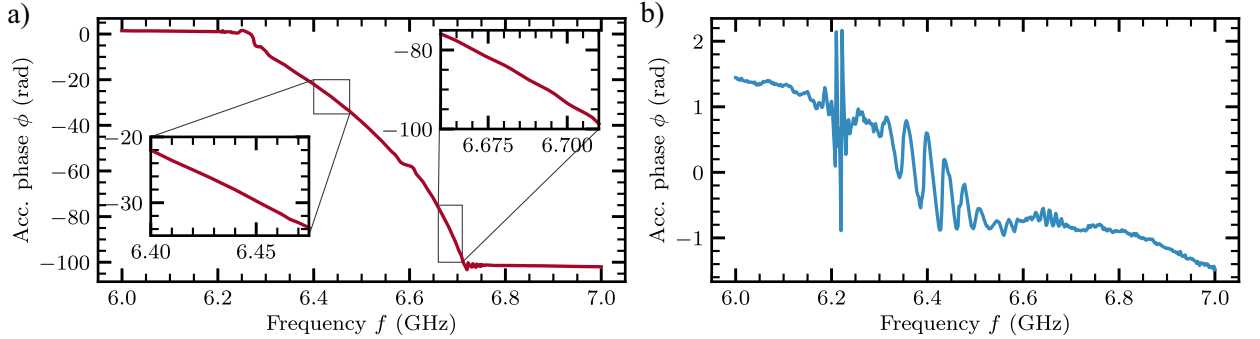

FIG. S7. Measured accumulated phases of the GS antenna and an external field of 143 mT for the  $S_{21}$  direction (a) and the  $S_{12}$  direction (b). Due to the strong spin-wave amplitude in the  $S_{21}$  trace, a strong phase accumulation is observed, that is only very slightly modulated by the interference with the EM. For the  $S_{12}$  trace with weak spin-wave amplitude, no significant phase accumulation is observed and a strong modulation due to the interference of spin-wave and EM contribution is measured.

## VI. BACK-ACTION ON THE DRIVING ANTENNA

The main text of the paper solely discusses the formation and influencing parameters of the passband ripple. However, the effects of the interference of EM and spin-wave signal are also detectable in the reflection at the input antenna. Similar to the transmission spectra, the dip in the reflection at the spin-wave resonance is distorted by



a frequency-dependent modulation. In a direct comparison of the two spectra, Figure S8 a) shows the course of both spectra for the GS antenna at 143 mT. Within the spin-wave band, it can be seen that both transmission and reflection are periodically modulated. The influence in the transmission is more pronounced and can be traced more clearly, qualitatively, however, the modulations match.

Similar to the observation in the main text for the transmission spectrum, a timegating procedure can also be used. As in the main text, the time evolution of the reflection is divided into two sections, one before the spin waves reach the detection antenna and one after. In contrast to the transmission spectrum, however, the undistorted response of the microwave network under consideration is not available for the reflection spectrum if only times at which the spin waves have already reached the detection antenna are taken into account. Instead, the undistorted case without back-action from the interference is only obtained if the times before the spin waves reach the detection antenna are explicitly considered. This is shown in Figure S8 b), in which only the first part of the time course is considered. In the filtered signal, the periodic distortions are removed.

The effective back-action of the spin waves at the output antenna to the excitation antenna is shown by the measurement of  $S_{11}$  as a measure of the total voltage wave returning to input port 1 of the VNA. Due to the phase offset of the voltages induced by the spin waves and EM and their frequency dependence, this results in a second voltage source in the entire network which, depending on the frequency, is in phase or out of phase with the oscillating voltage in the excitation antenna. If this contribution is effectively excluded in the time evolution, then no voltage source is present in the filtered system due to the spin waves and also not due to their interference with the EM in the detection antenna, meaning that they in turn cannot modulate the measured voltage at port 1.

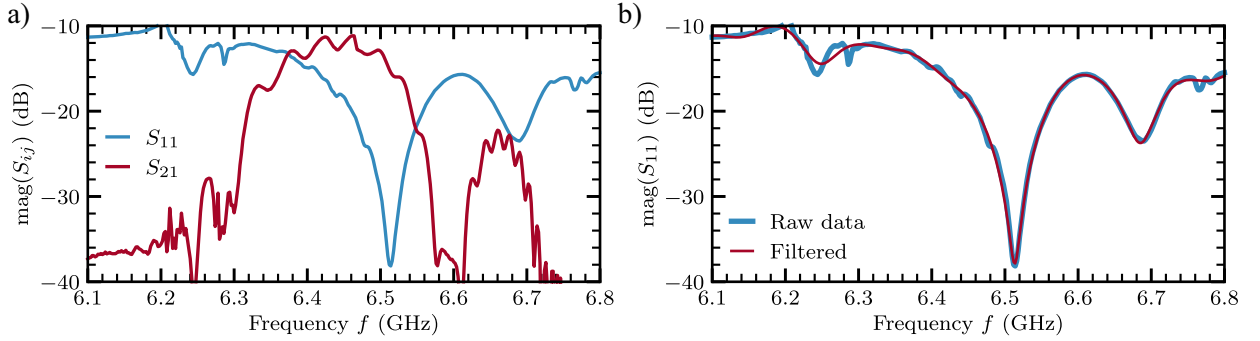

FIG. S8. a) Measured transmission and reflection spectrum for the GS antenna and an external field of 143 mT. b) Raw measured reflection spectrum along with the filtered spectrum. For the filtering only the first 13 ns, before the spin-waves reach the detection antenna, are considered. Filtering removes the distortions.

## VII. FURTHER ORIGINS OF RIPPLE FEATURES

The explanation of the modulations occurring in the reflection spectrum from Sec. VI is also valid without a direct influence of the interference of EM and spin waves propagating to the detection antenna. Rather, in the transformation necessary to calculate the  $S$ -parameters from the model:

$$S_{11} = \frac{(Z_{11} - Z_0)(Z_{22} + Z_0) - Z_{12} \cdot Z_{21}}{(Z_{22} + Z_0)(Z_{11} + Z_0) - Z_{12} \cdot Z_{21}},$$

$$S_{21} = \frac{2Z_0 Z_{21}}{(Z_{22} + Z_0)(Z_{11} + Z_0) - Z_{12} \cdot Z_{21}} \quad (\text{S5})$$

with  $Z_0 = 50 \Omega$  it can already be seen that in the reflection there is always a back-action of the dynamics in the detection antenna onto the reflection of the driving antenna caused by the term  $Z_{12} \cdot Z_{21}$ . These individual contributions, i.e. the spin waves and the EM, to the overall term  $Z_{12} \cdot Z_{21}$  can be estimated using the analytical model. In this model, the individual contributions to

$$Z_{ij} = Z_{ij,\text{sw}} + Z_{ij,\text{EM}} \quad (\text{S6})$$

can be scaled or adjusted separately and then the impact on the resulting reflection and transmission spectra can be identified. The results of the scaling obtained are plotted in Fig. S9. Here, black lines always describe the idealized

case, while a scaled impedance is assumed for the coloured lines (blue for reflection, red for transmission). In Fig. S9 a), the scenario with no EM interference is initially assumed. The reference case (black) for this consideration only assumes the native coupling impedances of the spin waves for the forward ( $Z_{21}$ ) and reverse ( $Z_{12}$ ) directions. Since the experiment is performed in the Damon-Eshbach configuration, which has a strong non-reciprocity (compare IV), the  $Z_{12}$  term is much smaller than the  $Z_{21}$  term. Thus, the effective feedback in the expression for  $S_{11}$  and  $S_{21}$  is small. This results in a smooth curve (black line in Fig. S9 a) ). However, if the  $Z_{12}$  term is scaled (factor 10) as for example in the case of backward-volume spin-waves, i.e. the feedback is amplified, clear periodic modulations occur in both  $S_{11}$  and  $S_{21}$ . Upon closer inspection, though, it is noticeable that the periodicity of these modulations is significantly shorter than that observed in the experiment. This observation can be understood with regard to the composition of the term  $Z_{12} \cdot Z_{21}$ . If the EM is omitted, both factors of the product show a phase development of

$$\phi = k(f) \cdot D \quad (\text{S7})$$

with the propagation distance  $D$ . Accordingly, the phase of the product revolves at double the speed, resulting in half the periodicity. Figuratively, the expression implies that the current in the excitation antenna excites spin waves, which in turn induce a current in the detection antenna. This current in turn excites spin waves, which travel the same way back to the excitation antenna and induce a current there. The effective propagation distance of these returning waves is therefore exactly twice as large as the distance  $D$  of the antennas. The coupling by spin waves alone in the experiment can therefore not explain the modulations that occur in reflection and transmission observed in the experiment.

Using the analytical model, this feedback of the spin waves can be completely eliminated in an idealized way. To do so,  $Z_{12}$  is artificially set to zero in the calculation. This case, without EM, is shown in black in Fig. S9 b). It shows smooth transmission and reflection spectra. If an inductive coupling by EM is now allowed in the calculation, for example  $Z_{ij,\text{EM}} = 5\Omega$ , the case of modulation by the interference of EM can be calculated without spin wave-induced feedback from the detection antenna to the excitation antenna. The results are shown by the colored lines in Fig. S9 b) assuming  $Z_{21,\text{EM}} = Z_{12,\text{EM}} = 5\Omega$ . Apparent modulations again occur in the spectra. However, since the EM is assumed to be frequency-independent, only the portion  $Z_{21,\text{sw}}$  contributes to the phase evolution of the coupling term. Consequently, the periodicity of the modulations is twice as large as in the case of pure spin-wave-moderated coupling and the modulation matching the experiment is obtained. In the experiment, due to the incomplete non-reciprocity of the spin waves, a mixed form of both considered cases is present, which can distort the observed modulations. This becomes more obvious for the reflection, as the coupling term appears in the numerator and denominator of Eq S5, while for the transmission parameters the pure  $Z_{ij}$  contributions dominate in the numerator. Therefore, the modulations of the reflections appear in Fig. S8 more distorted than for the transmission.

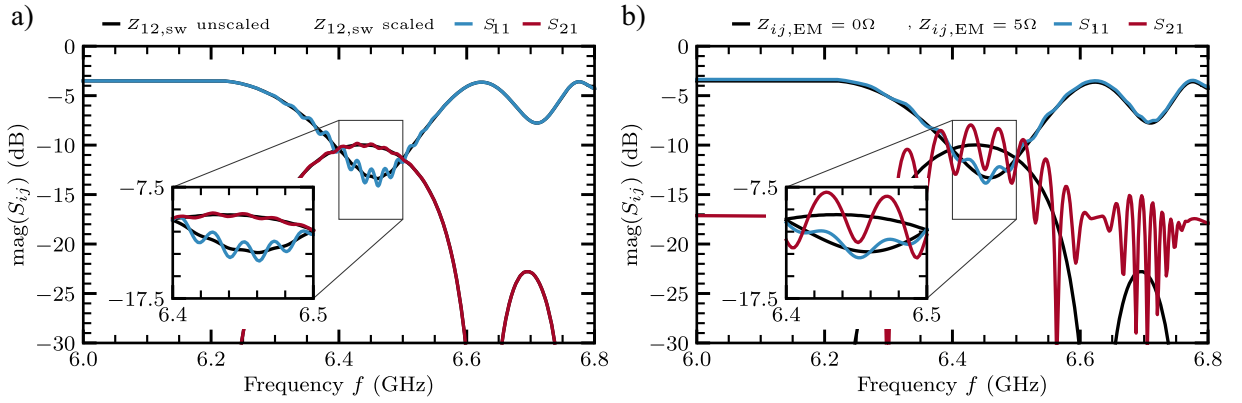

FIG. S9. a) Calculated transmission (red) and reflection (blue) spectrum for the GS antenna and an external field of 143 mT. Black lines refer to no EM and unscaled spin-wave impedances, while colored lines consider a scaled  $Z_{12}$ -contribution. b) Calculation for the same system as in a), considering  $Z_{12} = 0$  and no EM (black), while colored lines refer to EM impedance of  $5\Omega$ . Inset axis are zoom-ins for the transmission parameter. The electric resistance of the antenna is fixed to  $10\Omega$ .



- 
- [1] S. S. Kalarickal, P. Krivosik, M. Wu, C. E. Patton, M. L. Schneider, P. Kabos, T. J. Silva, and J. P. Nibarger, *Journal of Applied Physics* **99**, 093909 (2006).
  - [2] S. M. Rezende, *Fundamentals of Magnonics*, Lecture Notes in Physics, Vol. 969 (Springer International Publishing, Cham, 2020).
  - [3] F. Kohl, B. Heinz, Ádám Papp, R. Erdélyi, G. Csaba, and P. Pirro, “Identification and minimization of losses in microscaled spin-wave transducers,” (2025), [arXiv:2505.08656 \[physics.app-ph\]](#).
  - [4] D. Pozar, *Microwave Engineering* (Wiley, 2012).
  - [5] F. Vanderveken, V. Tyberkevych, G. Talmelli, B. Sorée, F. Ciubotaru, and C. Adelmann, *Scientific Reports* **12**, 3796 (2022).
  - [6] T. Devolder, G. Talmelli, S. Ngom, F. Ciubotaru, C. Adelmann, and C. Chappert, *Physical Review B* **103**, 214431 (2021).
